# Supplementary material for: Towards Prototype-Based Self-Explainable Graph Neural Network
Source: arXiv:2210.01974 source file (2022-10-05)
Supplement: Supplementary file 1 [file appendix.tex]

\appendix
\newpage
\section{Training Algorithm of {\method}}
\label{sec:algorithm}
The training algorithm of {\method} is given in Algorithm~\ref{alg:1}. In line 1, the parameters of the prototype generator $f_G$ and encoder $f_E$ initialized by pretraining with Eq.(\ref{eq:pretrain}) initialization. In
line 2, we obtain the initialized prototype graphs and the corresponding prototype embeddings based on the embeddings learned by the pretrained encoder. In line 4, we conduct prototype graph generation, which can be used to give predictions and two-levels of explanations. In line 5, the final loss function is computed. 
\begin{algorithm}[t] 
\caption{ Training Algorithm of {\method}.} 
\begin{algorithmic}[1]
\REQUIRE
$\mathcal{D}$, $K$, $M$, $T_l$, $T_h$, $\alpha$, $\beta$, $\tau$
\ENSURE $f_G$, $f_E$, $f_C$, and $\mathcal{\Tilde H}$.
\STATE Pretrain the $f_G$ and $f_E$ with Eq.(\ref{eq:pretrain})
\STATE Obtain the initialized prototypes and embeddings with Eq.(\ref{eq:get_init})
\REPEAT
\STATE Feed $\mathcal{\Tilde H}$ into the $f_G$ 
to generate the attributes and structure of  prototype graphs with $f_G$ by Eq.(\ref{eq:attr_dec}) and Eq.(\ref{eq:generate_graph})
\STATE Jointly optimize prototype embeddings  $\mathcal{\Tilde H}$ and the parameters of $f_G$ $f_E$, and $f_C$ by Eq.(\ref{eq:final})
\UNTIL convergence
\RETURN $f_G$, $f_E$, $f_C$, and $\mathcal{\Tilde H}$.
\end{algorithmic}
\label{alg:1}
\end{algorithm}

% \section{Impacts of the Number of Prototypes on Graph-SST2}
% See Figure~\ref{fig:nclu_app} for the additional experiments on Graph-SST2, which investigates the impacts of the number of prototypes on Graph-SST2. The observations are similar to those of Figure~\ref{fig:nclu}.
% \begin{figure}[h]
%     \small
%     \centering
%     \begin{subfigure}{0.49\linewidth}
%         \includegraphics[width=0.98\linewidth]{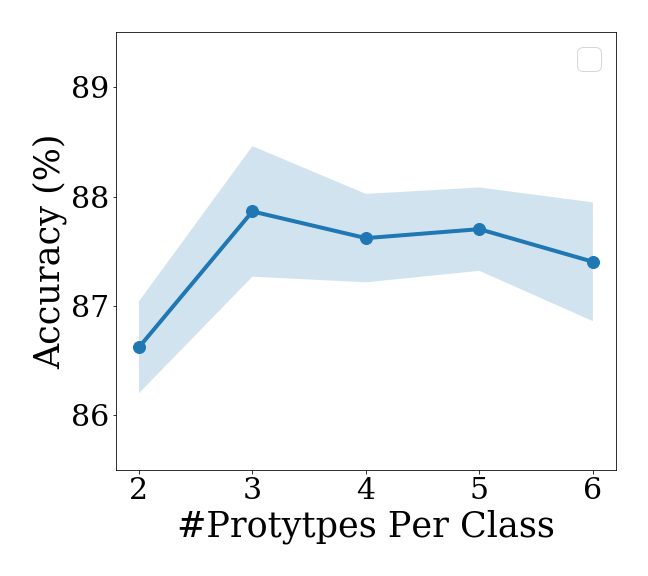}
%         \vskip -1em
%         \caption{Prediction Accuracy}
%     \end{subfigure}
%     \begin{subfigure}{0.49\linewidth}
%         \includegraphics[width=0.98\linewidth]{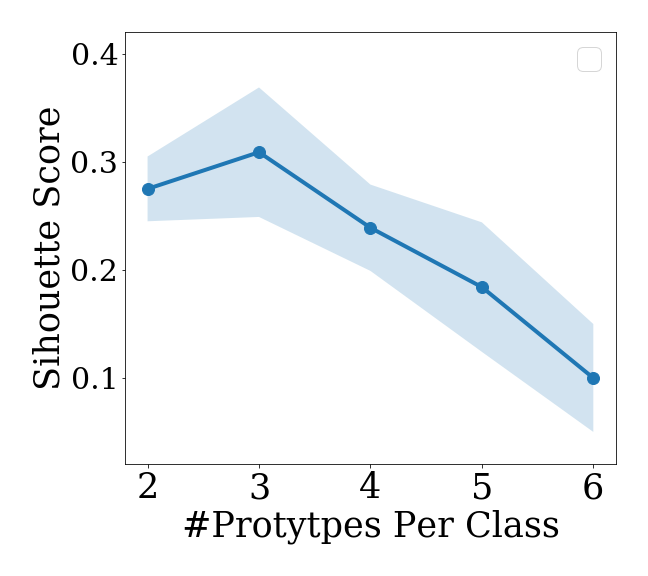}
%         \vskip -1em
%         \caption{Prototype Quality}
%     \end{subfigure}
%     \vskip -1.5em
%     \caption{The impacts of number of prototypes per class on graph classification dataset Graph-SST2.}
%     \vskip -1em
%     \label{fig:nclu_app}
% \end{figure}
% \label{sec:app_result}
